# Supplementary material for: Counterexample-Driven Synthesis for Probabilistic Program Sketches
Source: arXiv:1904.12371 source file (2019-04-28)
Supplement: Supplementary file 1 [file appendix.tex]

\clearpage\pagebreak
\appendix{}
[Whether we use the appendix in the end can be discussed later, just parking content here]
\subsection{Proof to sound and correct synthesiser}

In order to show completeness, observe that 	the synthesiser upon termination returns a conclusive answer. 
The synthesiser always terminates: 
In particular $\psi_{i+1} \not\vDash \alpha_i$, so after each iteration, there are strictly fewer models, and there are only finitely many models for $\psi_0$, so if the verifier always reports a conflict, the synthesiser eventually reports \texttt{Unsat}.
For soundness; the synthesiser only reports a realisation if the verifier reports that the realisation satisfies $\Phi$.
If the synthesiser reports \texttt{Unsat}, there is no realisation that satisfies $\Phi$. 
For contradiction, assume there was such a realisation $r^{*}$, and let $\alpha^{*}$ be the corresponding assignment to the corresponding meta-variables. 
Clearly, $\psi_0 \vDash \alpha^{*}$, and $\psi_n \not\vDash \alpha^{*}$. Thus, there exists a $j$ such that $\psi_{j} \vDash \alpha^{*}$ and $\psi_{j+1} \not\vDash \alpha^{*}$. 
 Thus, $\neg(\bigwedge_{h \in H, \bar{r}(h) \neq \bot} \kappa_h = \alpha_j(\kappa_h) ) \not \vDash \alpha_*$.
 
 \color{red}
 [ToDo ...finish..., show that $\bar{r}$ is not a conflict, which is a contradiction . ..]
 \color{black}
 
 \subsection{Proof to sound and correct verifier}
